# Supplementary material for: GRASP: Guiding model with RelAtional Semantics using Prompt for Dialogue Relation Extraction
Source: arXiv:2208.12494 source file (2022-09-27)
Supplement: Supplementary file 1 [file appendix.tex]

\appendix \label{appendix}

\section{Detailed experimental settings\label{appendix:experiment_settings}}
\input{tables/hyperparams}
$\mathbf{GRASP}$ is trained using AdamW\citep{loshchilov2017decoupled} as an optimizer with no weight decay. We set the number of training epochs as 30 with the early stopping, and the ratio of $\lambda_{1}$ and $\lambda_{2}$ for the joint loss as 0.7 to 0.3. We evaluate all of our model's performance by using a checkpoint which records the best F1 performance on the development set. We adopt the learning rate of $5e{-5}$, batch size of 8, and sequence length of 512 for RoBERTa-base, and $5e{-6}$, 8, and 512 for RoBERTa-large.

% related-works
\section{Related Works\label{appendix:related_works}}

\input{sections/1. related_works}
\input{tables/appen_qual1}
\section{Datasets and Baselines used in Analysis}\label{appendix:erc}
MELD is a multimodal dataset collected from TV shows and Friends. We only utilize textual modality in this dataset. It consists of seven emotion labels and 2,458 dialogues. 

EmoryNLP is also collected from the Friends. It is composed of seven emotion labels and 897 dialogues. Each utterance in these datasets is annotated with one of the seven emotion labels. We calculate weighted-F1 to evaluate MELD and EmoryNLP datasets.

COSMIC uses RoBERTa-large as an encoder. It is a framework that models various aspects of commonsense knowledge by considering mental states, events, actions, and cause-effect relations for emotional recognition in conversations. 
\section{Qualitative Analysis Examples\label{appendix:qualitative}}
Table \ref{table:appen_qual1} shows additional examples to demonstrate the prediction tendency of $\mathbf{GRASP}$ and the fine-tuned RoBERTa models on symmetrical relation described in \ref{subsec:qualitative}.
